# Supplementary material for: Optical induced Spin Current in Monolayer NbSe$_2$
Source: arXiv:2105.03021 source file (2021-05-07)
Supplement: Supplementary file 1 [file Supplementary_material.pdf]

# Supplementary material for "Optical induced Spin Current of Monolayer $NbSe_2$"


Ren Habara[1] and Katsunori Wakabayashi[1,2,3]

[1]*Department of Nanotechnology for Sustainable Energy, School of Science and Technology, Kwansei Gakuin University, Gakuen 2-1, Sanda 669-1337, Japan*

[2]*National Institute for Materials Science (NIMS), Namiki 1-1, Tsukuba 305-0044, Japan*

[3]*Center for Spintronics Research Network (CSRN), Osaka University, Toyonaka 560-8531, Japan*


# Matrix Elements of Monolayer $NbSe_2$

We employ a multi-orbitals tight-binding model (TBM) which includes $d_{z^2}$, $d_{x^2-y^2}$ and $d_{xy}$ orbitals of Nb atom to describe the electronic states of $NbSe_2$. [1–3] The eigenvalue equation for TBM is $\hat{H}(\boldsymbol{k})|u_{n\boldsymbol{k}}\rangle = E_{n\boldsymbol{k}}|u_{n\boldsymbol{k}}\rangle$, where $\boldsymbol{k} = (k_x, k_y)$ is the wavenumber vector, $E_{n\boldsymbol{k}}$ is the eigenvalue and $n = 1, 2, \cdots, 6$ is the band index. The eigenvector is defined as $|u_{n\boldsymbol{k}}\rangle = (c_{n\boldsymbol{k},d_{z^2},\uparrow}, c_{n\boldsymbol{k},d_{xy},\uparrow}, c_{n\boldsymbol{k},d_{x^2-y^2},\uparrow}, c_{n\boldsymbol{k},d_{z^2},\downarrow}, c_{n\boldsymbol{k},d_{xy},\downarrow}, c_{n\boldsymbol{k},d_{x^2-y^2},\downarrow})^T$, where $(\cdots)^T$ indicates the transpose of vector and $c_{n\boldsymbol{k}\tau s}$ means the amplitude at atomic orbital $\tau$ with spin $s$ for the $n$th energy band at $\boldsymbol{k}$. The Hamiltonian with the SOC can be written as

$$\hat{H}(\boldsymbol{k}) = \hat{\sigma}_0 \otimes \hat{H}_{TNN}(\boldsymbol{k}) + \hat{\sigma}_z \otimes \frac{1}{2}\lambda_{SOC}\hat{L}_z \tag{1}$$

with

$$\hat{H}_{TNN}(\boldsymbol{k}) = \begin{pmatrix} V_0 & V_1 & V_2 \\ V_1^* & V_{11} & V_{12} \\ V_2^* & V_{12}^* & V_{22} \end{pmatrix} \tag{2}$$

and

$$\hat{L}_z = \begin{pmatrix} 0 & 0 & 0 \\ 0 & 0 & -2i \\ 0 & 2i & 0 \end{pmatrix}. \tag{3}$$

Here, $\hat{\sigma}_0$ and $\hat{\sigma}_z$ are Pauli matrices, and $\lambda_{SOC}$ is Ising-type SOC parameter. In monolayer $NbSe_2$, $\lambda_{SOC} = 0.0784$ eV. $\hat{H}_{TNN}(\boldsymbol{k})$ includes electron hoppings only among three $d$-orbitals of Nb atoms, which are assumed up to third-nearest neighbor sites as shown in Supplementary Fig. 1 (a). Here, green, red and blue arrows indicate hopping vectors $\boldsymbol{R_i}$ $(i = 1, 2, \cdots, 6)$ pointing to nearest-neighbor (n.n) sites, the vectors $\tilde{\boldsymbol{R}}_{\boldsymbol{j}}$ $(j = 1, 2, \cdots, 6)$ pointing to next n.n sites and the vectors $2\boldsymbol{R_i}$ pointing to third n.n sites, respectively. We can find the matrix elements in the effective TBM Hamiltonian: $V_0$, $V_1$, $V_2$, $V_{11}$, $V_{12}$ and $V_{22}$ as

$$V_0 = \varepsilon_1 + 2t_0(2\cos\alpha\cos\beta + \cos 2\alpha) + 2r_0(2\cos 3\alpha\cos\beta + \cos 2\beta) + 2u_0(2\cos 2\alpha\cos 2\beta + \cos 4\alpha), \tag{4}$$

$$\mathrm{Re}[V_1] = -2\sqrt{3}t_2\sin\alpha\sin\beta + 2(r_1 + r_2)\sin 3\alpha\sin\beta - 2\sqrt{3}u_2\sin 2\alpha\sin 2\beta, \tag{5}$$

$$\mathrm{Im}[V_1] = 2t_1\sin\alpha(2\cos\alpha + \cos\beta) + 2(r_1 - r_2)\sin 3\alpha\cos\beta + 2u_1\sin 2\alpha(2\cos 2\alpha + \cos 2\beta), \tag{6}$$

$$\mathrm{Re}[V_2] = 2t_2(\cos 2\alpha - \cos\alpha\cos\beta) - \frac{2}{\sqrt{3}}(r_1 + r_2)(\cos 3\alpha\cos\beta - \cos 2\beta) + 2u_2(\cos 4\alpha - \cos 2\alpha\cos 2\beta), \tag{7}$$

$$\mathrm{Im}[V_2] = 2\sqrt{3}t_1\cos\alpha\sin\beta + \frac{2}{\sqrt{3}}(r_1 - r_2)\sin\beta(\cos 3\alpha + 2\cos\beta) + 2\sqrt{3}u_1\cos 2\alpha\sin 2\beta, \tag{8}$$

$$\begin{aligned} V_{11} = \varepsilon_2 &+ (t_{11} + 3t_{22})\cos\alpha\cos\beta + 2t_{11}\cos 2\alpha + 4r_{11}\cos 3\alpha\cos\beta \\ &+ 2(r_{11} + \sqrt{3}r_{12})\cos 2\beta + (u_{11} + 3u_{22})\cos 2\alpha\cos 2\beta + 2u_{11}\cos 4\alpha, \end{aligned} \tag{9}$$

$$\mathrm{Re}[V_{12}] = \sqrt{3}(t_{22}-t_{11})\sin\alpha\sin\beta + 4r_{12}\sin 3\alpha\sin\beta + \sqrt{3}(u_{22}-u_{11})\sin 2\alpha\sin 2\beta, \tag{10}$$

$$\mathrm{Im}[V_{12}] = 4t_{12}\sin\alpha(\cos\alpha-\cos\beta) + 4u_{12}\sin 2\alpha(\cos 2\alpha-\cos 2\beta), \tag{11}$$

$$\begin{aligned} V_{22} = {} & \varepsilon_2 + (3t_{11}+t_{22})\cos\alpha\cos\beta + 2t_{22}\cos 2\alpha + 2r_{11}(2\cos 3\alpha\cos\beta + \cos 2\beta) \\ & + \frac{2}{\sqrt{3}}r_{12}(4\cos 3\alpha\cos\beta - \cos 2\beta) + (3u_{11}+u_{22})\cos 2\alpha\cos 2\beta + 2u_{22}\cos 4\alpha. \end{aligned} \tag{12}$$

Here, $(\alpha,\beta) = (\frac{1}{2}k_x a, \frac{\sqrt{3}}{2}k_y a)$ and the lattice constant $a$ is 3.45 Å. The specific hopping parameters in this TBM can be given as

$$E^{jj'}_{\mu\mu'}(\boldsymbol{R}) = \langle \psi^j_\mu(\boldsymbol{r})|\hat{H}(\boldsymbol{k})|\phi^{j'}_{\mu'}(\boldsymbol{r}-\boldsymbol{R})\rangle, \tag{13}$$

where $|u_{n\boldsymbol{k}}\rangle \to \left|\phi^j_\mu\right\rangle$ indicates an atomic orbital of Nb atom and in this paper, we consider $\left|\phi^1_1\right\rangle = d_{z^2}$, $\left|\phi^2_1\right\rangle = d_{xy}$ and $\left|\phi^2_2\right\rangle = d_{x^2-y^2}$. For example, we can express $t_0 = E^{11}_{11}(\boldsymbol{R_1})$, $t_1 = E^{12}_{11}(\boldsymbol{R_1})$, $r_0 = E^{11}_{11}(\tilde{\boldsymbol{R}}_1)$, $r_1 = E^{12}_{11}(\tilde{\boldsymbol{R}}_1)$, $u_0 = E^{11}_{11}(2\boldsymbol{R_1})$ and $u_1 = E^{12}_{11}(2\boldsymbol{R_1})$. The details about fitted parameters for this TBM are summarized in Supplementary Table 1, [1] and the corresponding energy band structure and density of states (DOS) are shown in Supplementary Fig. 1 (b). Here, red and blue lines indicate spin-up and spin-down states. The shape of the energy band structure is qualitatively similar to heavily hole-doped monolayer $MoS_2$. Unlike monolayer $MoS_2$ which shows semiconducting behavior, monolayer $NbSe_2$ is metallic, but a large energy band gap between the partially filled valence bands and empty conduction bands. Also, the Ising-type SOC provides opposite spin splitting at the valence band edges in K and K′ points, and time-reversal symmetry protection. In particular, at the K point, the SOC makes the spin splitting about 157 meV.

Supplementary Table 1. Fitting parameters for the effective TBM Hamiltonian of monolayer $NbSe_2$. The energy parameters $\varepsilon_1$ to $\lambda_{SOC}$ are in units of eV.

| $\varepsilon_1$ | $\varepsilon_2$ | $t_0$ | $t_1$ | $t_2$ | $t_{11}$ | $t_{12}$ | $t_{22}$ | $r_0$ | $r_1$ |
|---|---|---|---|---|---|---|---|---|---|
| $r_2$ | $r_{11}$ | $r_{12}$ | $u_0$ | $u_1$ | $u_2$ | $u_{11}$ | $u_{12}$ | $u_{22}$ | $\lambda_{SOC}$ |
| 1.4466 | 1.8496 | -0.2308 | 0.3116 | 0.3459 | 0.2795 | 0.2787 | -0.0539 | 0.0037 | -0.0997 |
| 0.0385 | 0.0320 | 0.0986 | 0.0685 | -0.0381 | 0.0535 | 0.0601 | -0.0179 | -0.0425 | 0.0784 |

# Comparison between Spin Berry Curvature and Charge Berry Curvature

As shown in Fig. 2 (a) in main text, the spin Berry curvature clearly shows the six-fold symmetry in the first Brillouin Zone (BZ). However, for each spin state, the symmetry with respect to Γ point reduces to three-fold symmetry. This is because monolayer $NbSe_2$ possesses opposite spin splitting around K and K′ points, i.e., anisotropic energy band structure.

The spin Berry curvature is given as

$$\Omega^{spin}(\boldsymbol{k}) = \hbar\sum_n f(E_{n\boldsymbol{k}})\sum_{m\neq n}\frac{-2\mathrm{Im}\,\langle u_{n\boldsymbol{k}}|\hat{j}^{spin}_x|u_{m\boldsymbol{k}}\rangle\,\langle u_{m\boldsymbol{k}}|\hat{v}_y|u_{n\boldsymbol{k}}\rangle}{(E_{m\boldsymbol{k}}-E_{n\boldsymbol{k}})^2}, \tag{14}$$

where the details of notation are given in main text. Since Ising-type SOC does not couple up-spin states with down-spin states, the Hamiltonian is always block diagonalized as for the spin sector, i.e., Eq. (1) can be expressed as

$$\hat{H}(\boldsymbol{k}) = \begin{pmatrix} \hat{H}^{\uparrow} & 0 \\ 0 & \hat{H}^{\downarrow} \end{pmatrix}, \tag{15}$$

where $\hat{H}^{\uparrow}$ ($\hat{H}^{\downarrow}$) is the Hamiltonian solely for up-spin (down-spin) states. Thus, we can separate the spin Berry curvature into the contributions of each spin state, i.e., we can define as

$$\Omega^{spin}(\boldsymbol{k}) = \frac{\Omega^{\uparrow}(\boldsymbol{k}) - \Omega^{\downarrow}(\boldsymbol{k})}{2}. \tag{16}$$

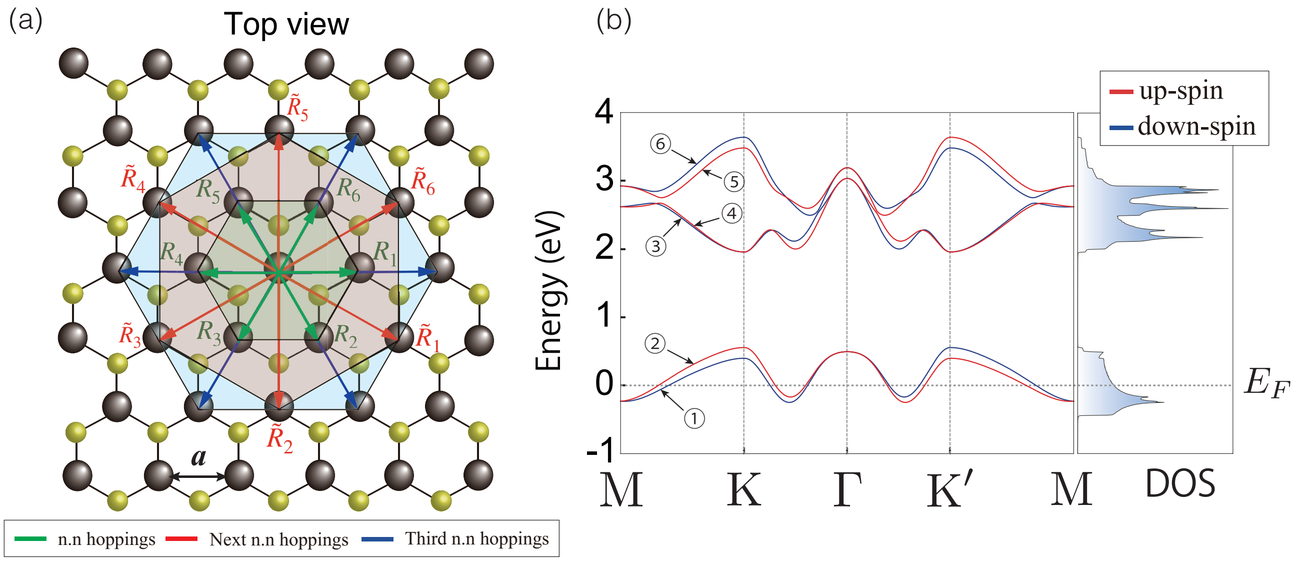


Supplementary Figure 1. (a) Top view of crystal structure of monolayer $NbSe_2$ which consists of Nb (black) and Se (yellow) atoms. Green, red and blue arrows indicate hopping vectors $\boldsymbol{R_i}$ $(i = 1, 2, \cdots, 6)$ pointing to n.n sites, the vectors $\tilde{\boldsymbol{R}}_{\boldsymbol{j}}$ $(j = 1, 2, \cdots, 6)$ pointing to next n.n sites and the vectors $2\boldsymbol{R_i}$ pointing to third n.n sites, respectively. $a$ is the lattice constant. (b) Energy band structure and DOS of $NbSe_2$ with SOC parameter $\lambda_{SOC} = 0.0784$ eV. Fermi level is set to zero. Monolayer $NbSe_2$ with SOC includes six energy bands ① to ⑥. Here, ②, ④ and ⑤ indicate the energy bands of spin-up states. On the other hand, ①, ③ and ⑥ indicate the energy bands of spin-down states.

Here, $\Omega^{\uparrow}(\boldsymbol{k})$ is the Berry curvature solely for spin-up state, which can be written as

$$\Omega^{\uparrow}(\boldsymbol{k}) = \hbar^2 \sum_n f(E^{\uparrow}_{n\boldsymbol{k}}) \sum_{m\neq n} \frac{-2\mathrm{Im}\,\langle u^{\uparrow}_{n\boldsymbol{k}}|\hat{v}^{\uparrow}_x|u^{\uparrow}_{m\boldsymbol{k}}\rangle\,\langle u^{\uparrow}_{m\boldsymbol{k}}|\hat{v}^{\uparrow}_y|u^{\uparrow}_{n\boldsymbol{k}}\rangle}{(E^{\uparrow}_{m\boldsymbol{k}} - E^{\uparrow}_{n\boldsymbol{k}})^2}. \tag{17}$$

Here $|u^{\uparrow}_{n\boldsymbol{k}}\rangle = (c_{n\boldsymbol{k},d_{z^2},\uparrow}, c_{n\boldsymbol{k},d_{xy},\uparrow}, c_{n\boldsymbol{k},d_{x^2-y^2},\uparrow})^T$, $(\hat{v}^{\uparrow}_x, \hat{v}^{\uparrow}_y) = \frac{1}{\hbar}(\frac{\partial H^{\uparrow}}{\partial x}, \frac{\partial H^{\uparrow}}{\partial y})$, and $E^{\uparrow}_{n\boldsymbol{k}}$ is the eigenenergy of $\hat{H}^{\uparrow}$. In similar manner, we can define $\Omega^{\downarrow}(\boldsymbol{k})$, which is the Berry curvature solely for down-spin state, as

$$\Omega^{\downarrow}(\boldsymbol{k}) = \hbar^2 \sum_n f(E^{\downarrow}_{n\boldsymbol{k}}) \sum_{m\neq n} \frac{-2\mathrm{Im}\,\langle u^{\downarrow}_{n\boldsymbol{k}}|\hat{v}^{\downarrow}_x|u^{\downarrow}_{m\boldsymbol{k}}\rangle\,\langle u^{\downarrow}_{m\boldsymbol{k}}|\hat{v}^{\downarrow}_y|u^{\downarrow}_{n\boldsymbol{k}}\rangle}{(E^{\downarrow}_{m\boldsymbol{k}} - E^{\downarrow}_{n\boldsymbol{k}})^2}. \tag{18}$$

Supplementary Figures 2 (a) and (b) shows the contour plot for $\Omega^{\uparrow}(\boldsymbol{k})$ and $\Omega^{\downarrow}(\boldsymbol{k})$, respectively. It is clearly seen that both of them has three-hold symmetry not six-hold symmetry.

In further, we can give the charge Berry curvature as

$$\Omega^{charge}(\boldsymbol{k}) = \Omega^{\uparrow}(\boldsymbol{k}) + \Omega^{\downarrow}(\boldsymbol{k}) \tag{19}$$

$$= \hbar^2 \sum_n f(E_{n\boldsymbol{k}}) \sum_{m\neq n} \frac{-2\mathrm{Im}\,\langle u_{n\boldsymbol{k}}|\hat{v}_x|u_{m\boldsymbol{k}}\rangle\,\langle u_{m\boldsymbol{k}}|\hat{v}_y|u_{n\boldsymbol{k}}\rangle}{(E_{m\boldsymbol{k}} - E_{n\boldsymbol{k}})^2}. \tag{20}$$

Supplementary Figure 2 (c) shows the charge Berry curvature which is plotted along the path passing through high-symmetric points of 1st BZ. The Berry curvature has the anti-symmetric peak around Γ point. Supplementary Figure 2 (d) shows the two-dimensional (2D) contour plot of charge Berry curvature in 1st BZ and the three-fold symmetry. Thus, the charge Berry curvature has odd parity, i.e., $\Omega^{charge}(\boldsymbol{k}) = -\Omega^{charge}(-\boldsymbol{k})$. Therefore the charge Hall conductivity becomes identically zero, i.e.,

$$\sigma^{charge}_{xy} \sim \sum_{\boldsymbol{k}} \Omega^{charge}(\boldsymbol{k}) = 0. \tag{21}$$

Thus, the pure spin current can be induced by light irradiation in monolayer $NbSe_2$.

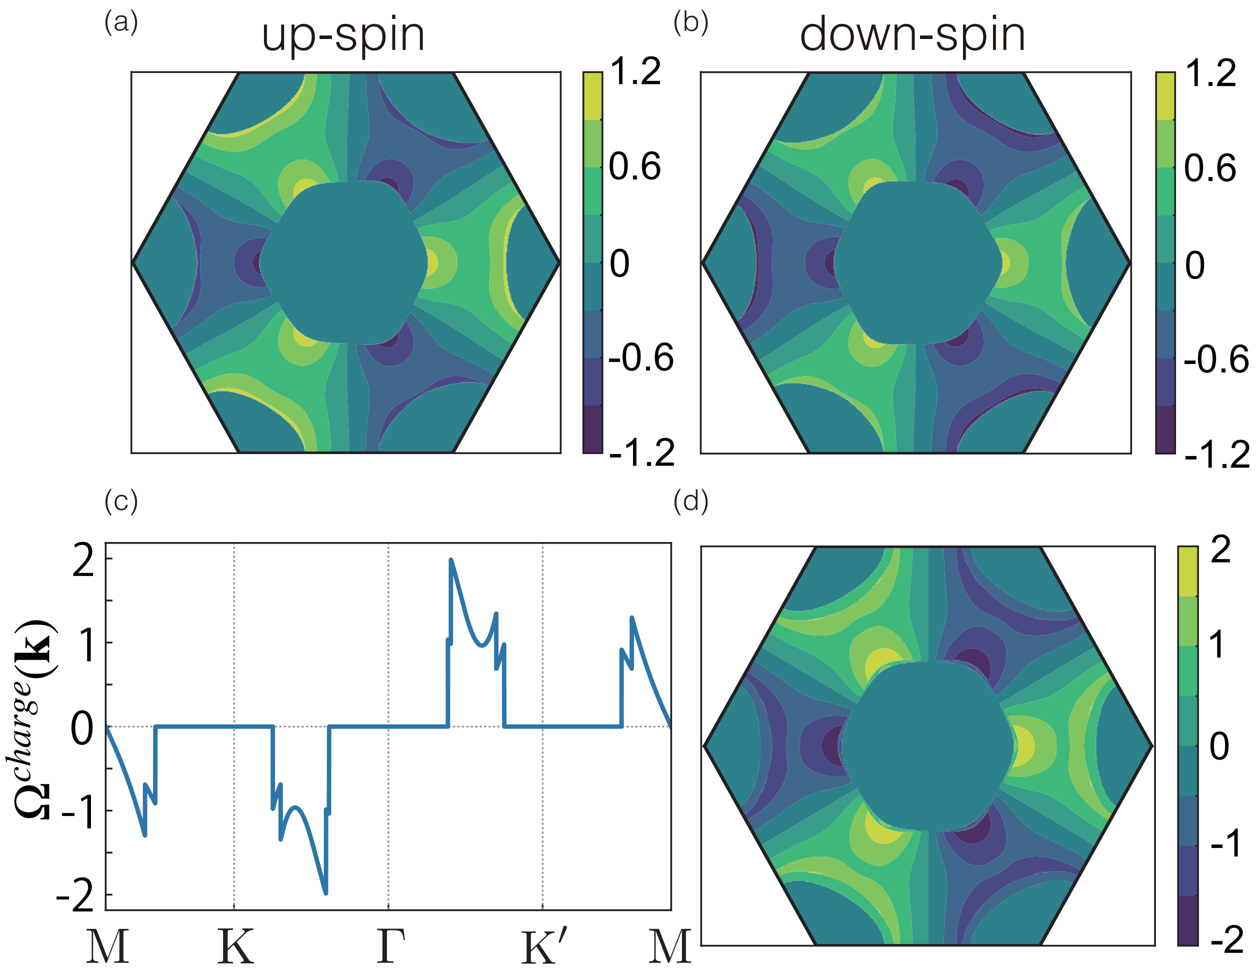


Supplementary Figure 2. Berry curvature of (a) up-spin and (b) down-spin states with SOC parameter $\lambda_{SOC} = 0.0784$ eV. Charge Berry curvature of monolayer $NbSe_2$ with SOC parameter $\lambda_{SOC} = 0.0784$ eV. (c) Plot along the path through the high-symmetric points in 1st BZ. (d) Contour plot in 1st BZ.

# Spin-Dependent Optical Hall Conductivity for Each Transition to Different Conduction Bands

In this paper, we can obtain optical angular frequency dependence of spin-dependent Hall conductivity taking into account transitions to the conduction bands which are the energy bands ③ to ⑥ [see Supplementary Figure 3 (a)]. The Hall conductivity has large peak around 3.0 eV under light irradiation. However, the result does not reveal that which transition to different conduction bands leads to the maximum of spin-dependent optical Hall conductivity, so that we investigate the conductivity for each transition to different conduction bands. Here, we consider two transitions to conduction bands (lower conduction bands ③, ④ and larger conduction bands ⑤, ⑥) in the energy band structure. Supplementary Figure 3 (b) indicates spin-dependent optical Hall conductivity for transitions to ③, ④ and does not correspond to the peak of Supplementary Fig. 3 (a). On the other hand, Supplementary Figure 3 (c) indicates spin-dependent optical Hall conductivity for transitions to ⑤, ⑥ and corresponds to the peak of Supplementary Fig. 3 (a). These results are obvious to attribute peak of the corresponding DOS of monolayer $NbSe_2$.

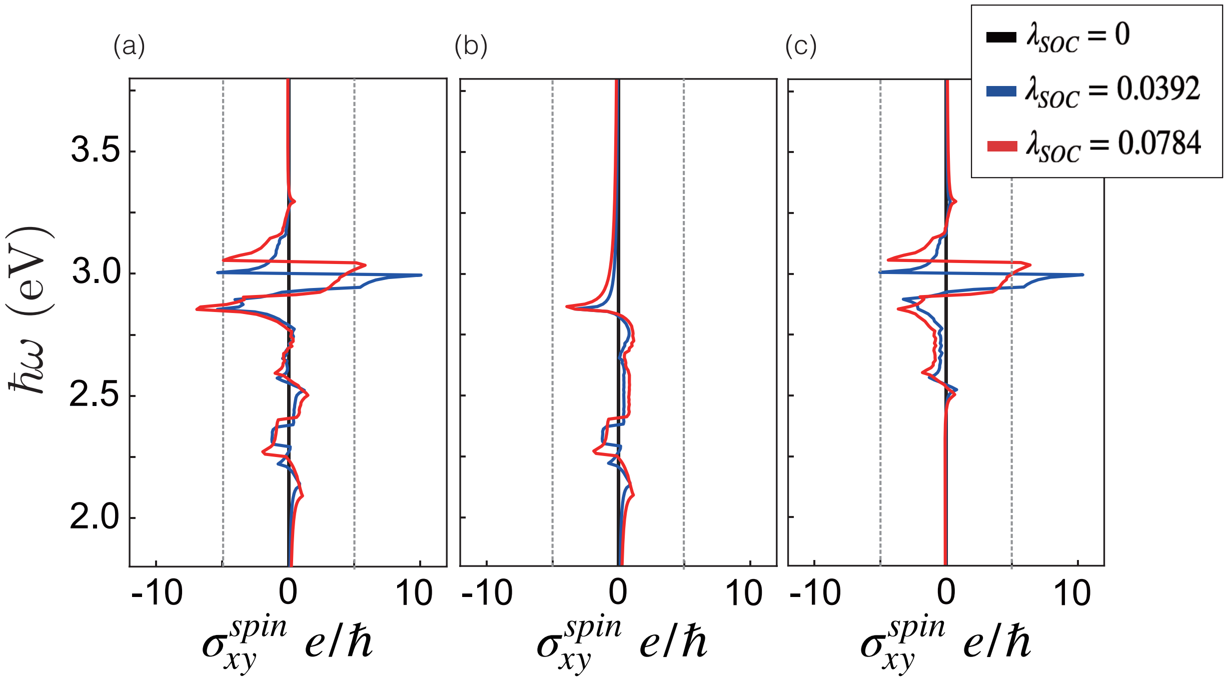


Supplementary Figure 3. Optical angular frequency dependence of spin-dependent Hall conductivity $\sigma_{xy}^{spin}(\omega)$ for transitions to (a) conduction bands ③ to ⑥, (b) conduction bands ③, ④ and (c) conduction bands ⑤, ⑥. Black, blue and red lines indicate several different SOC parameters. The unit of $\sigma_{xy}^{spin}(\omega)$ is $e^2/\hbar$.

# Spin Berry Curvature of Electron-Doped Monolayer $NbSe_2$

When electrons are doped into monolayer $NbSe_2$, monolayer $NbSe_2$ shows semiconducting behavior as same as monolayer $MoS_2$ [4–6]. Supplementary Figure 4 (a) indicates spin Berry curvature [7–16] of the electron-doped monolayer $NbSe_2$ along high symmetry lines of 1st BZ and unlike non-doped monolayer $NbSe_2$, it has maximum at K and K′ points. In Supplementary Fig. 4 (b), the spin Berry curvature has six-fold symmetry around Γ point, so that spin-dependent Hall conductivity which is the summation of the spin Berry curvature over the momentum is nonvanishing. On the other hand, charge Berry curvature can be written as Eq. (17) and possesses opposite sign at K and K′ points [see Supplementary Figure 4 (c)]. Here, Supplementary Figure 4 (c) indicates the charge Berry curvature which is plotted along the path passing through high-symmetric points of 1st BZ. The Berry curvature has the anti-symmetric peak at K and K′ points. Supplementary Figure 4 (d) shows the 2D contour plot of charge Berry curvature in 1st BZ and the three-fold symmetry. As the result, the charge Hall conductivity is vanished in 2D momentum space, so that we can generate pure spin Hall current accompanied by valley current [6, 17].

# Temperature Dependence of Spin-Dependent Hall Conductivity and Optical Longitudinal Conductivity

Supplementary Figure 5 (a) shows temperature dependence of spin-dependent Hall conductivity of monolayer $NbSe_2$ with SOC parameter $\lambda_{SOC} = 0.0784$ eV. The effect of optical induced spin Hall current is robust to temperature, and is expected to be observed even in room temperature. As the result, we can use monolayer $NbSe_2$ for the application of *spin current harvesting* by irradiation light in visible and ultraviolet range.

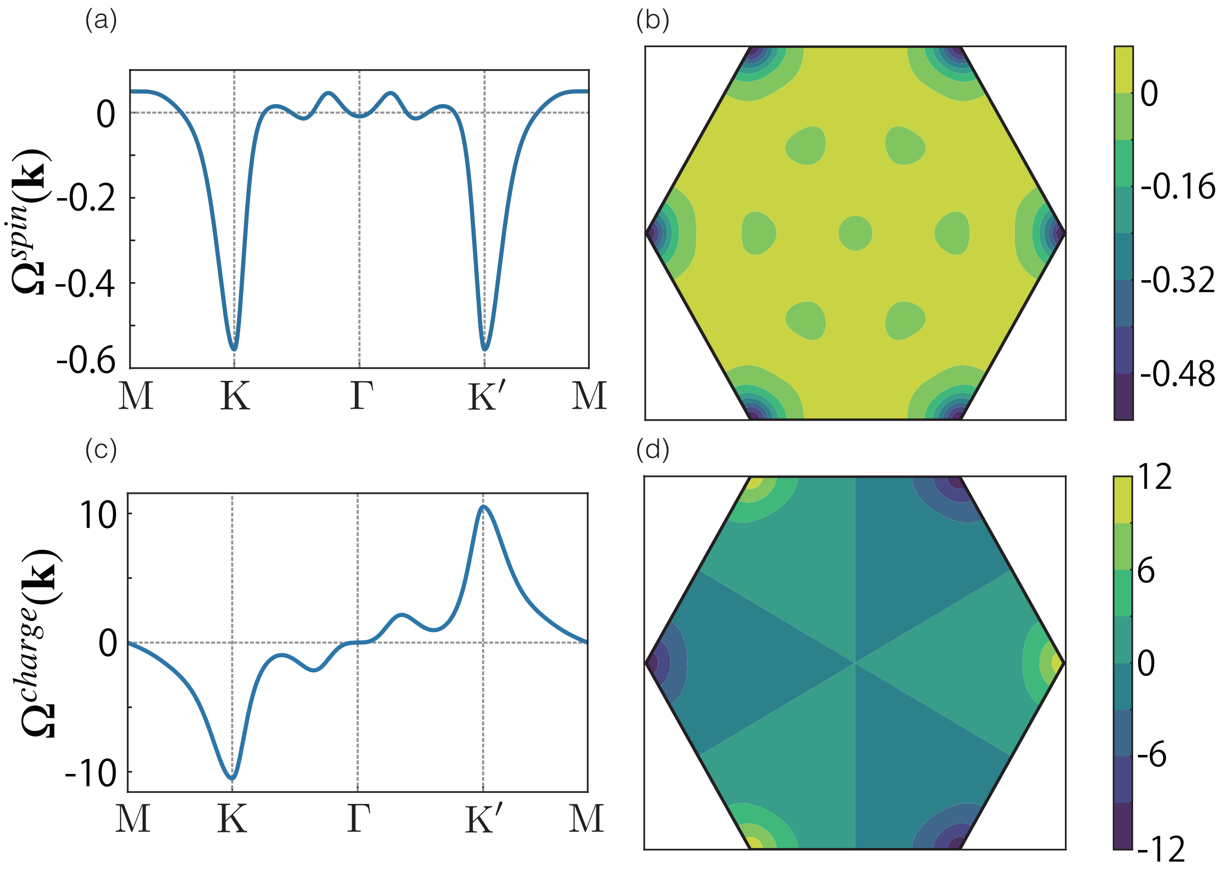


Supplementary Figure 4. Spin Berry curvature of electron-doped monolayer $NbSe_2$ with SOC parameter $\lambda_{SOC} = 0.0784$ eV (a) along high symmetry lines of 1st BZ and (b) in 2D momentum space. Charge Berry curvature of electron-doped monolayer $NbSe_2$ with the same as SOC parameter as the spin Berry curvature. (c) Plot along the path through the high-symmetric points in 1st BZ. (d) Contour plot in 1st BZ.

In order to evaluate spin Hall angle (SHA), [7, 16, 18–20] we introduce optical longitudinal conductivity [21–23]

$$\sigma_{xx}(\omega) = -\frac{i\hbar e^2}{S}\sum_{\boldsymbol{k}}\sum_{nm}\frac{f(E_{n\boldsymbol{k}}) - f(E_{m\boldsymbol{k}})}{E_{m\boldsymbol{k}} - E_{n\boldsymbol{k}}}\frac{|\langle u_{m\boldsymbol{k}}|\hat{v}_x|u_{n\boldsymbol{k}}\rangle|^2}{E_{m\boldsymbol{k}} - E_{n\boldsymbol{k}} - \hbar\omega - i\eta}. \tag{22}$$

Here, $n(m)$ indicates the band index, $|u_{n\boldsymbol{k}}\rangle$ is the eigen function with the eigen energy $E_{n\boldsymbol{k}}$, $f(E_{n\boldsymbol{k}})$ is Fermi-Dirac distribution function, and $\hat{v}_x$ is a group velocity operator. Supplementary Figure 5 (b) is a result of the conductivity for several different SOC parameters and is similar to the shape of DOS of monolayer $NbSe_2$. Also, the conductivity has large peak around 3.0 eV under light irradiation. Here, the unit of the optical longitudinal conductivity is $e^2/\hbar$.

# Spin-Dependent Optical Hall Conductivity of Electron- or Hole-Doped Monolayer $NbSe_2$

The spin-dependent optical Hall conductivity [6–8, 22, 24–28] can be given as

$$\sigma_{xy}^{spin}(\omega) = \frac{i\hbar e}{S}\sum_{\boldsymbol{k}}\sum_{nm}\frac{f(E_{n\boldsymbol{k}}) - f(E_{m\boldsymbol{k}})}{E_{m\boldsymbol{k}} - E_{n\boldsymbol{k}}}\frac{\langle u_{n\boldsymbol{k}}|\hat{j}_x^{spin}|u_{m\boldsymbol{k}}\rangle\langle u_{m\boldsymbol{k}}|\hat{v}_y|u_{n\boldsymbol{k}}\rangle}{E_{m\boldsymbol{k}} - E_{n\boldsymbol{k}} - \hbar\omega - i\eta}. \tag{23}$$

Here, $\hat{j}_x^{spin}$ is spin current operator and written as $\hat{j}_x^{spin} = \frac{1}{2}\{\frac{\hbar}{2}\hat{\sigma}_z \otimes \hat{I}_3, \hat{v}_x\}$, where $\hat{I}_3$ is the $3\times 3$ identity matrix and $\hat{v}_{x(y)}$ is the group velocity operator. $\sigma_{xy}^{spin}(\omega)$ is a function of Fermi level, so that we calculate new $\sigma_{xy}^{spin}(\omega)$ obtained by shifting the

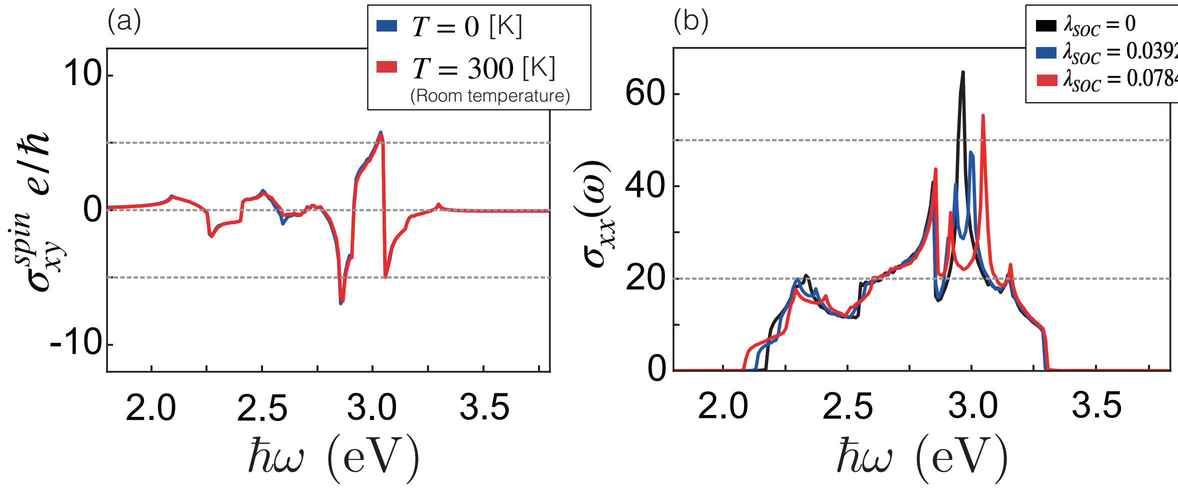


Supplementary Figure 5. (a) Temperature dependence of spin-dependent Hall conductivity $\sigma_{xy}^{spin}(\omega)$ of monolayer $NbSe_2$ with SOC parameter $\lambda_{SOC} = 0.0784$ eV. Blue and red lines indicate absolute and room temperature, respectively. (b) Optical longitudinal conductivity $\sigma_{xx}(\omega)$ of monolayer $NbSe_2$ for several different SOC parameters. The units of $\sigma_{xy}^{spin}(\omega)$ and $\sigma_{xx}(\omega)$ are $e^2/\hbar$.

Fermi level position. For hole-doped monolayer $NbSe_2$, monolayer $NbSe_2$ is metallic and the calculated $\sigma_{xy}^{spin}(\omega)$ as shown in Supplementary Fig. 6 (b) can get lower peak than the result of the non-doped monolayer $NbSe_2$ [see Supplementary Figure 6 (a)]. This indicates that owing to shifting down the Fermi level, the number of states in the partially filled valence bands decreases, so the conductivity totally becomes lower. On the other hand, for electron-doped monolayer $NbSe_2$, we can provide the results for two different Fermi levels. Firstly, when we set $E_F = 0.3$ eV, monolayer $NbSe_2$ is still metallic and the calculated $\sigma_{xy}^{spin}(\omega)$ as shown in Supplementary Fig. 6 (c) can obtain its maximum around 3.0 eV under light irradiation. Also, unlike non-doped monolayer $NbSe_2$, the conductivity shows larger value around 2.3 eV under light irradiation. Next, when we set $E_F = 1.0$ eV, monolayer $NbSe_2$ becomes semiconductor and the calculated $\sigma_{xy}^{spin}(\omega)$ as shown in Supplementary fig. 6 (d) can obtain largest value in Suppelmentary Fig. 6. These results indicate that owing to shifting up the Fermi level, the number of states in the partially filled valence bands increases, so the conductivity totally becomes larger. However, according to the corresponding DOS of monolayer $NbSe_2$, the number of states which have increased almost exclusively contributes to the interband transitions of lower energy around 2.3 eV. As the result, the conductivity shows a large change around 2.3 eV by light irradiation, so that the pure spin current can be enhanced by electron-doping.

[1] W.-Y. He, B. T. Zhou, J. J. He, N. F. Q. Yuan, T. Zhang, and K. T. Law, Commun. Phys. **1**, 40 (2018).
[2] G.-B. Liu, W.-Y. Shan, Y. Yao, W. Yao, and D. Xiao, Phys. Rev. B **88**, 085433 (2013).
[3] S. Kim and Y.-W. Son, Phys. Rev. B **96**, 155439 (2017).
[4] X. Li and H. Zhu, J. Materiomics **1**, 33 (2015).
[5] W. Feng, Y. Yao, W. Zhu, J. Zhou, W. Yao, and D. Xiao, Phys. Rev. B **86**, 165108 (2012).
[6] Z. Li and J. P. Carbotte, Phys. Rev. B **86**, 205425 (2012).
[7] J. Qiao, J. Zhou, Z. Yuan, and W. Zhao, Phys. Rev. B **98**, 214402 (2018).
[8] Y. Yao, L. Kleinman, A. H. MacDonald, J. Sinova, T. Jungwirth, D.-s. Wang, E. Wang, and Q. Niu, Phys. Rev. Lett. **92**, 037204 (2004).
[9] J. Sławińska, F. T. Cerasoli, H. Wang, S. Postorino, A. Supka, S. Curtarolo, M. Fornari, and M. B. Nardelli, 2D Mater. **6**, 025012 (2019).
[10] Y. Yao and Z. Fang, Phys. Rev. Lett. **95**, 156601 (2005).
[11] H. Da, Q. Song, P. Dong, H. Ye, and X. Yan, J. Appl. Phys. **127**, 023903 (2020).
[12] M. Gradhand, D. V. Fedorov, F. Pientka, P. Zahn, I. Mertig, and B. L. Györffy, J. Phys. Condens. Matter **24**, 213202 (2012).
[13] G. Qu, K. Nakamura, and M. Hayashi, arXiv:1901.05651 (2019).
[14] J. Kim, K.-W. Kim, D. Shin, S.-H. Lee, J. Sinova, N. Park, and H. Jin, Nat. Commun. **10**, 3965 (2019).
[15] G. Y. Guo, S. Murakami, T.-W. Chen, and N. Nagaosa, Phys. Rev. Lett. **100**, 096401 (2008).
[16] J. Zhou, J. Qiao, A. Bournel, and W. Zhao, Phys. Rev. B **99**, 060408 (2019).
[17] W.-Y. Shan, J. Zhou, and D. Xiao, Phys. Rev. B **91**, 035402 (2015).
[18] S. Y. Huang, D. Qu, T. C. Chuang, C. C. Chiang, W. Lin, and C. L. Chien, Appl. Phys. Lett. **117**, 190501 (2020).
[19] Y. Wang, P. Deorani, X. Qiu, J. H. Kwon, and H. Yang, Appl. Phys. Lett. **105**, 152412 (2014).
[20] W. Zhang, W. Han, S.-H. Yang, Y. Sun, Y. Zhang, B. Yan, and S. S. P. Parkin, Sci. Adv. **2**, e1600759 (2016).

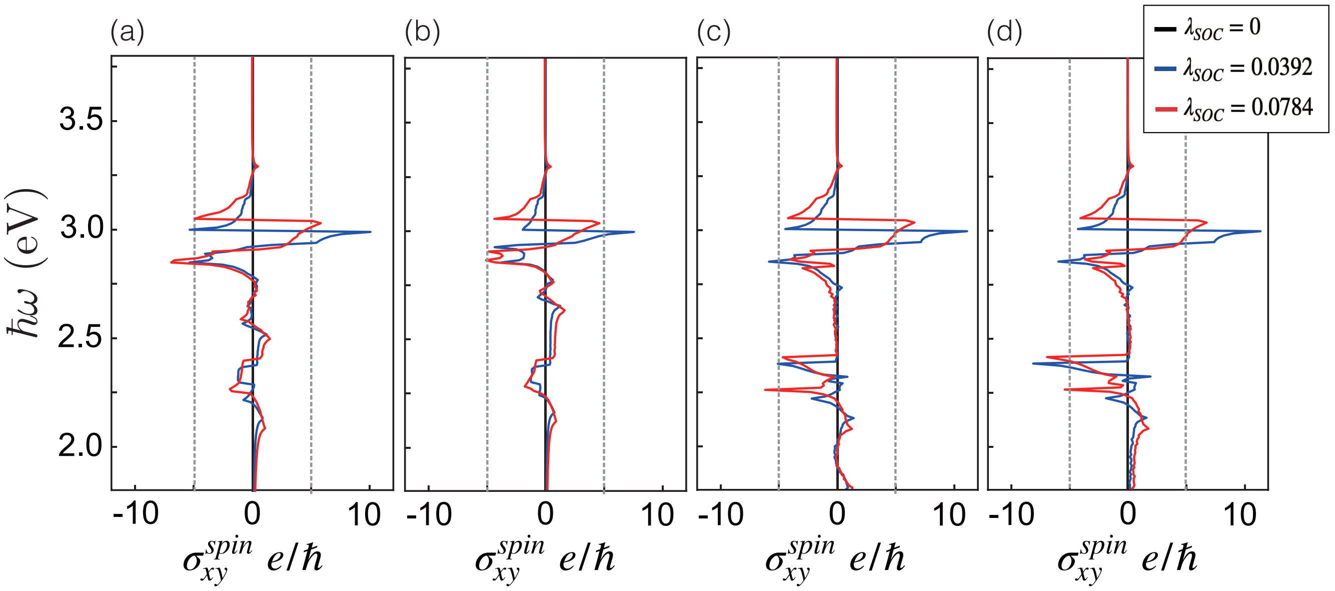


Supplementary Figure 6. Optical angular frequency dependence of spin-dependent Hall conductivity $\sigma_{xy}^{spin}(\omega)$ of (a) $E_F = 0$ eV, (b) $E_F = -0.1$ eV, (c) $E_F = 0.3$ eV and (d) $E_F = 1.0$ eV for several different SOC parameters. The unit of $\sigma_{xy}^{spin}(\omega)$ is $e^2/\hbar$.


[21] R. Kubo, J. Phys. Soc. Japan **12**, 570 (1957).
[22] A. Ferreira, J. Viana-Gomes, Y. V. Bludov, V. Pereira, N. M. R. Peres, and A. H. C. Neto, Phys. Rev. B **84**, 235410 (2011).
[23] S. Saberi-Pouya, T. Vazifehshenas, T. Salavati-fard, M. Farmanbar, and F. M. Peeters, Phys. Rev. B **96**, 075411 (2017).
[24] G. Y. Guo, Y. Yao, and Q. Niu, Phys. Rev. Lett. **94**, 226601 (2005).
[25] P. Sengupta, S. Rakheja, and E. Bellotti, arXiv:1512.06734 (2015).
[26] V. Vargiamidis, P. Vasilopoulos, and G.-Q. Hai, J. Phys. Condens. Matter **26**, 345303 (2014).
[27] T. Tanaka, H. Kontani, M. Naito, T. Naito, D. S. Hirashima, K. Yamada, and J. Inoue, Phys. Rev. B **77**, 165117 (2008).
[28] T. Morimoto, Y. Hatsugai, and H. Aoki, Phys. Rev. Lett. **103**, 116803 (2009).
